# Supplementary material for: Spectroscopic signatures of biexcitons: A case study in Ruddlesden-Popper lead-halides
Source: arXiv:2503.11890 source file (2025-03-14)
Supplement: Supplementary file 1 [file SI_2Qpaper.pdf]

# Supporting Information: Spectroscopic signatures of biexcitons: A case study in Ruddlesden-Popper lead-halides

Katherine A. Koch,[1] Esteban Rojas-Gatjens,[2] Martín Gómez-Dominguez,[3] Juan-Pablo Correa-Baena,[3] Carlos Silva-Acuña,[2,3,4] and Ajay Ram Srimath Kandada[1,*]

[1]*Department of Physics and Center for Functional Materials, 2090 Eure Drive, Wake Forest University, Winston-Salem, NC 27109, United States*

[2]*School of Chemistry and Biochemistry, Georgia Institute of Technology, 901 Atlantic Drive, Atlanta, GA 30332, United States*

[3]*School of Materials Science and Engineering, Georgia Institute of Technology, 771 Ferst Dr NW, Atlanta, GA 30332, United States*

[4]*Institut Courtois & Département de Physique, Université de Montréal, 1375 Avenue Thérèse-Lavoie-Roux, Montréal H2V 0B3, Québec, Canada*

(Dated: March 14, 2025)

## A. Sample Preparation

Glass slides were cleaned using sequential ultrasonic baths of acetone and isopropanol (IPA) for 15 minutes each, followed by nitrogen drying and UV-ozone treatment for 15 minutes. The perovskite precursor solutions were prepared by dissolving equimolar amounts of $PbI_2$ (purity >99.99%) and the corresponding organic cation, 4F-phenethylammonium iodide (purity >99.99%), in N,N-dimethylformamide (purity >99.98%) at a concentration of 0.13 M. After stirring overnight, the perovskite films were deposited by dispensing 80 $\mu$L of the precursor solution onto a 2.54 $cm^2$ clean glass slide, then spin-coated at 6000 RPM for 30s with an acceleration of 6000 RPM/s. Immediately after deposition, the films were thermally annealed at 100°C for 10 minutes.

## B. Two-Dimensional Electronic Spectroscopy (2DES)

We employed 2D spectroscopy on $(F-PEA)_2PbI_4$ using the previously implemented scheme [1, 2], developed and described in detail by Turner and coworkers [3]. The pulses used for these measurements were generated by a home-built single pass non-collinear optical parametric amplifier pumped by the third harmonic of a Yb:KGW ultrafast laser system (Pharos Model PH1-20-0200-02-10, Light Conversion) emitting 1030-nm pulses at 100kHz, with an output power of 20 W and pulse duration of 220-fs. The pulses were individually compressed using a home-built implementation of a pulse shaper using a chirp scan [4]. The resulting pulse duration was 25 fs full-width at half-maximum (FWHM), as measured by second-harmonic generation cross-frequency-resolved optical gating (SHG-XFROG). All measurements were carried out in a vibration-free closed-cycle cryostat (Montana Instruments).

## C. Binding Energy Estimations

### 1. *Photoluminluminescence*

To estimate the biexciton binding energy from the photoluminesence spectra, we fit the data using a double Guassian function to determine the peak positions of the two resonances (see Fig. S1 and S2). The energy difference between the two resonances provides an estimate of the biexciton binding energy, shown in Fig. 5(c).

### 2. *2DES: One-Quantum (1Q)*

To estimate the biexciton binding energy from the 1Q rephasing spectra, we need to determine the peak position of the excited state absorption feature (ESA). We performed a gradient calculation of the absolute 1Q spectra and took the magnitude of the gradient to find the position of the peak's maximum. The position of this feature was utilized to estimate the biexciton binding energy, see Fig. S3.

### 3. *2DES: Two-Quantum (2Q)*

To estimate the biexciton binding energy from the 2Q non-rephasing spectra, we utilized gradient analysis to get more accurate estimations of the feature positions. Figure S4(c), shows the vertical slice, taken at the energy (2.32 eV) of the main diagonal feature in the gradient map, where the difference between twice the cut energy (red dashed line) and the peak position of the vertical slice (red solid line) provides the estimation of the binding energy.

The mixed biexciton binding energy ($E_{B_{12}}$) is determined from the experimental 2Q absolute spectra. The diagonal feature is $\sim$ 33 meV below the energy of the average of the two-quantum energies for $X_1$ and $X_2$, see Fig. S4(a).

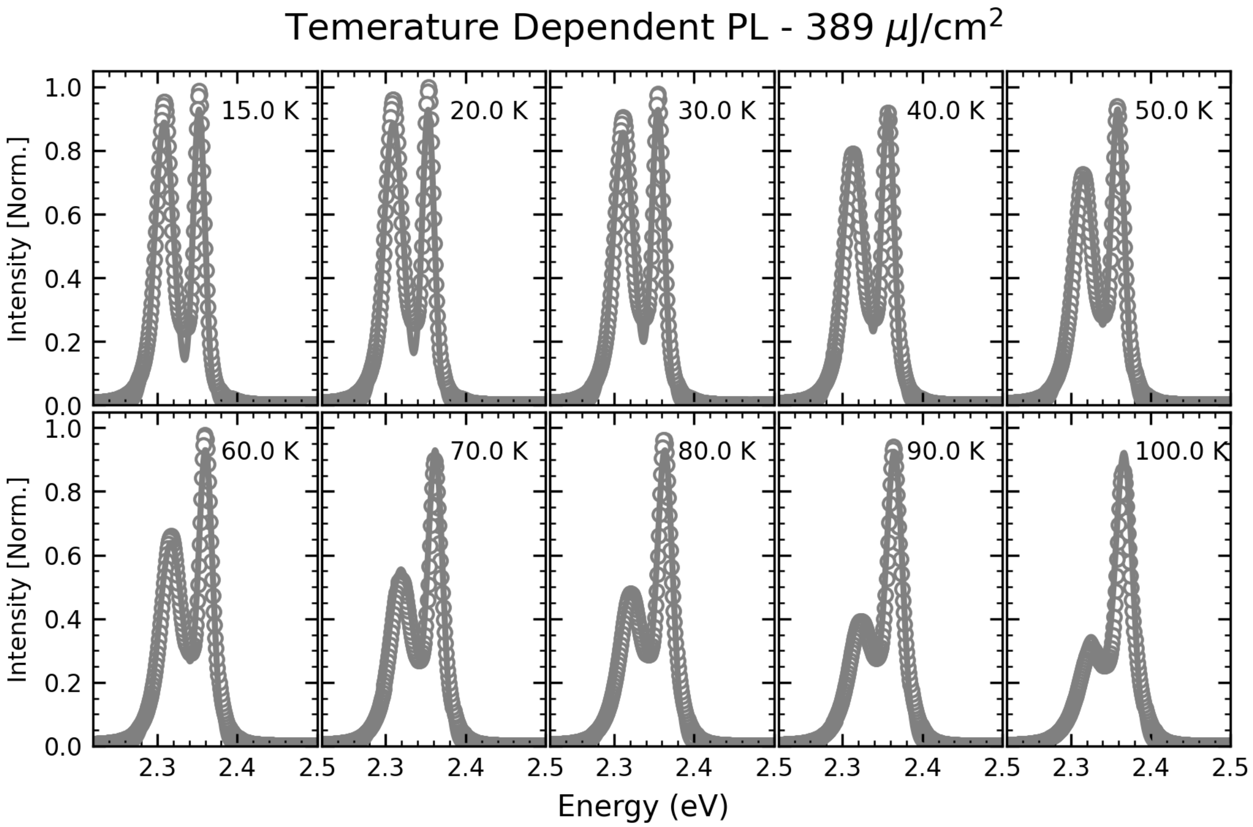


FIG. S1. Temperature dependent photoluminesence spectra (dots) fit to a double Guassian function (lines). The measurements are performed with a excitation energy of 2.95 eV (420 nm) and a fluence of 389 $\mu$J/cm$^2$.

### D. Two-Quantum (2Q) analytical expressions

$$S^{\Sigma_1} = -\sum_i \frac{|\mu_{gX_i}|^2 |\mu_{X_iB_i}|^2}{(i(\omega_2 - \omega_{B_ig}) - \Gamma_{B_ig})\,(i(\omega_3 - \omega_{B_iX_i}) - \Gamma_{B_iX_i})} \tag{1}$$

$$S^{\Sigma_2} = \sum_i \frac{|\mu_{gX_i}|^2 |\mu_{X_iB_i}|^2}{(i(\omega_2 - \omega_{B_ig}) - \Gamma_{B_ig})\,(i(\omega_3 - \omega_{gX_i}) - \Gamma_{gX_i})} \tag{2}$$

$$S^{\Sigma_3} = -\sum_{i\neq j} \frac{|\mu_{gX_i}|^2 |\mu_{B_{ij}X_i}|^2}{(i(\omega_2 - \omega_{B_{ij}g}) - \Gamma_{B_{ij}g})(i(\omega_3 - \omega_{B_{ij}X_i}) - \Gamma_{B_{ij}X_1}))} \tag{3}$$

$$S^{\Sigma_4} = \sum_{i\neq j} \frac{|\mu_{gX_i}|^2 |\mu_{B_{ij}X_i}|^2}{(i(\omega_2 - \omega_{B_{ij}g}) - \Gamma_{B_{ij}g})(i(\omega_3 - \omega_{gX_i}) - \Gamma_{gX_1}))} \tag{4}$$

* srimatar@wfu.edu

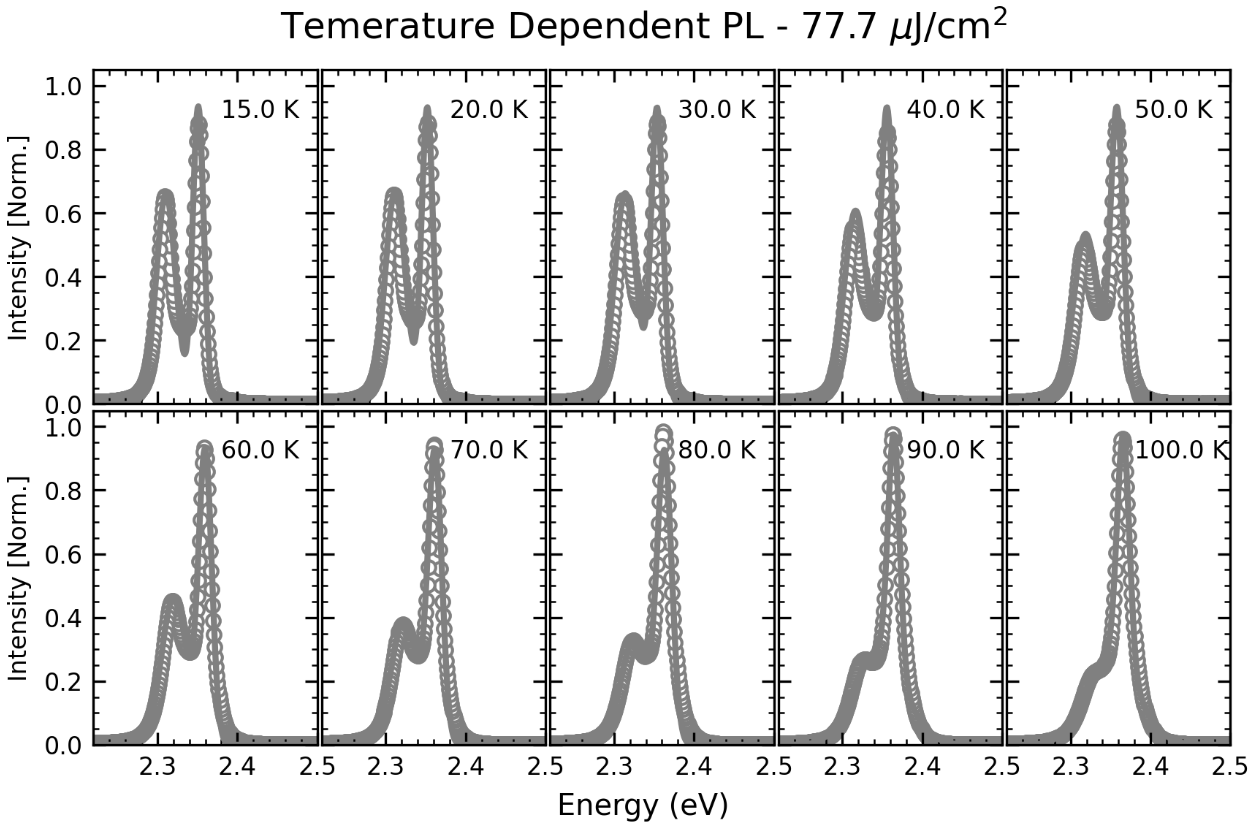


FIG. S2. Temperature dependent photoluminesence spectra (dots) fit to a double Guassian function (lines). The measurements are performed with a excitation energy of 2.95 eV (420 nm) and a fluence of 77.7 $\mu$J/cm$^2$.

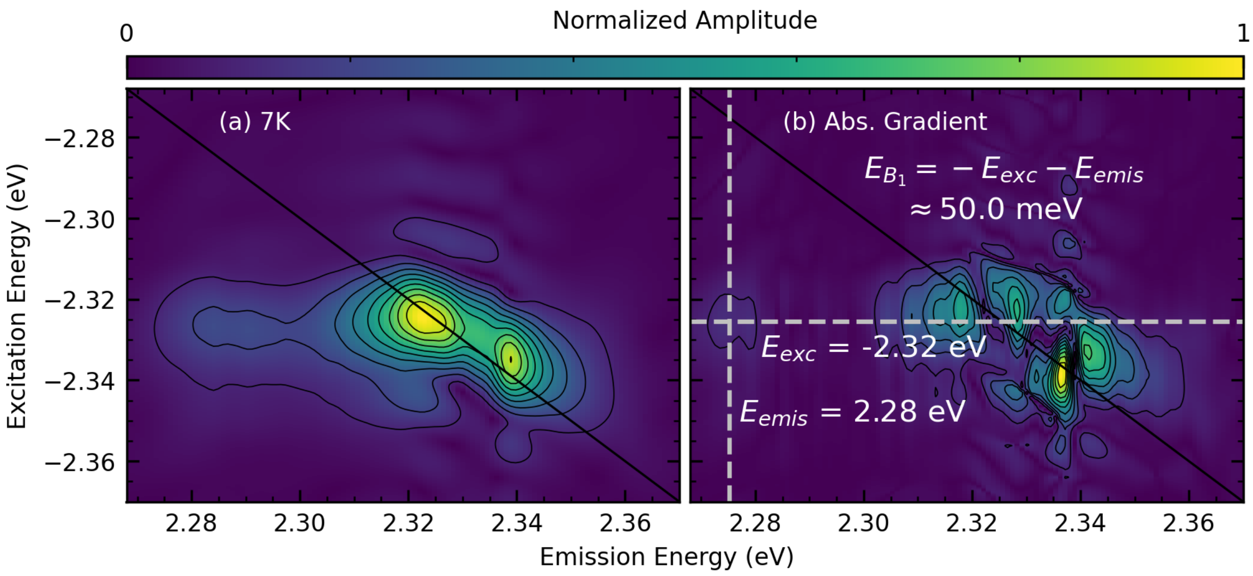


FIG. S3. (a) Absolute one-quantum rephasing 2DES spectrum measured at 7K. (b) Absolute gradient of the 1Q spectra shown in (a), where the biexciton binding energy was estimated from the ESA peak.

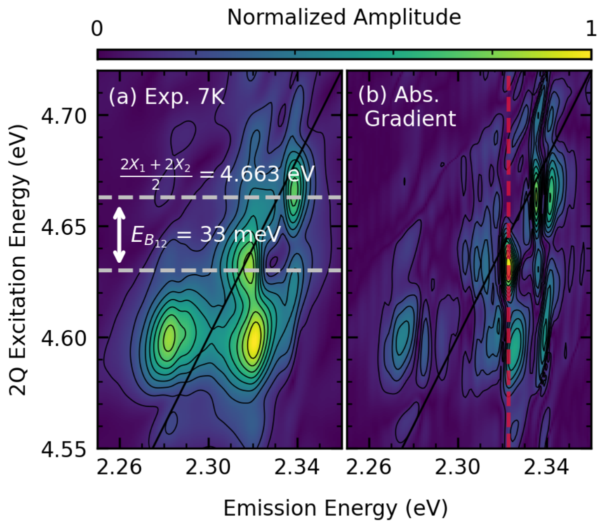


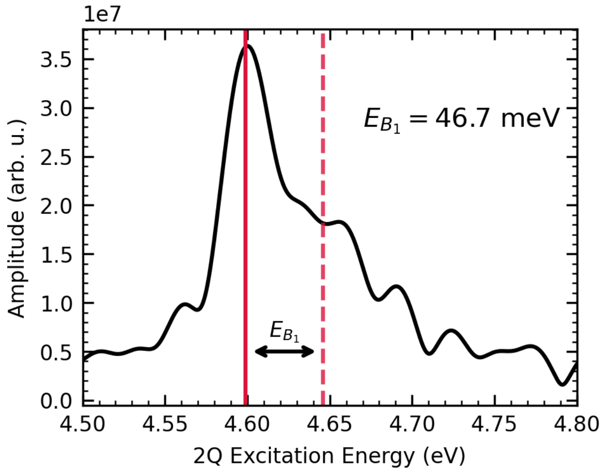


FIG. S4. (a) Absolute two-quantum non-rephasing 2DES spectrum measured at 7K. (b) Absolute gradient of the 2Q spectra shown in (a). (c) A vertical slice of the 2Q absolute gradient map, taken at 2.32 eV (red dashed line in (b)), where the dashed red line in (c) represents twice the cut energy (4.64 eV). The biexciton binding energy is estimated as the difference between twice the cut energy (red dashed line) and the peak position of the vertical slice (red solid line).


[1] F. Thouin, S. Neutzner, D. Cortecchia, V. A. Dragomir, C. Soci, T. Salim, Y. M. Lam, R. Leonelli, A. Petrozza, A. R. S. Kandada, *et al.*, Physical Review Materials **2**, 034001 (2018).

[2] F. Thouin, D. Cortecchia, A. Petrozza, A. R. Srimath Kandada, and C. Silva, Physical Review Research **1**, 032032 (2019).

[3] D. B. Turner, K. W. Stone, K. Gundogdu, and K. A. Nelson, Review of Scientific Instruments **82** (2011).

[4] V. Loriot, G. Gitzinger, and N. Forget, Optics Express **21**, 24879 (2013).
